# Supplementary material for: VideoJudge: Bootstrapping Enables Scalable Supervision of MLLM-as-a-Judge for Video Understanding
Source: arXiv:2509.21451 source file (2025-09-25)
Supplement: Supplementary file 1 [file evaluation_data_appendix.tex]

\subsection{Evaluation}\label{subsec:evaluation}
% Our evaluation framework combines both pointwise and pairwise settings to provide a comprehensive assessment of judge models. Pointwise evaluation measures how well models assign meaningful scores to individual responses, enabling fine-grained analysis through correlation and error metrics. Pairwise evaluation, on the other hand, captures relative preferences by comparing two responses for the same video--instruction pair, with accuracy reported against human or rating-based ground truth. Together, these complementary approaches offer a holistic view of model performance across diverse evaluation benchmarks.

We evaluate judge models in two complementary settings. Pointwise evaluation measures whether a model can assign meaningful scores to individual responses, while pairwise evaluation tests whether it can consistently prefer the better of two responses to the same instruction and align well with human or ground-truth ratings.

\subsubsection{Pointwise Evaluation}  
In pointwise evaluation, each video--instruction--response triplet is judged independently, with the model producing a reasoning trace followed by a quality rating. This setup directly measures a model’s ability to assign meaningful scores to individual responses. The explicit integer ratings provide fine-grained evaluation, enabling correlation analysis and error metrics to capture both the consistency and reliability of the judgments.

\paragraph{VideoJudge-Pointwise}  
We construct two benchmarks for pointwise evaluation: \textbf{VideoJudgeLLaVA-MetaEval} and \textbf{VideoJudgeVCG-MetaEval}. For VideoJudgeLLaVA-MetaEval, we source videos, instructions, and initial gold-standard responses from LLaVA~\cite{}, while for VideoJudgeVCG-MetaEval we use JudgeVCG~\cite{}. In both cases, additional candidate responses are generated using our bootstrapping pipeline (Algorithm~\ref{alg:bootstrap}) with an acceptance threshold of $0$ to ensure consistency between the evaluator and generator models. We then manually inspect examples to ensure that responses and ratings are properly aligned, resulting in 5,000 high-quality meta-evaluation examples for each benchmark. Each video--instruction--response triplet is gas with a single integer rating on a 1--5 scale, and our evaluation prompts require models to produce reasoning followed by ratings in this format. Importantly, both the videos and instructions in these evaluation datasets are out-of-distribution, and we confirm that no near-duplicates were found. We report divergence error alongside correlation metrics.

\paragraph{Vatex-Eval~\citep{shi2022emscoreevaluatingvideocaptioning}}
The Vatex-Eval benchmark consists of videos paired with captioning instructions and candidate captions. Each candidate is annotated by multiple evaluators, and the final ground-truth score is the average of these judgments. Because these scores are continuous values that reflect aggregated human preferences, our evaluation focuses on metrics that capture whether models assign higher ratings to preferred captions and lower ratings to less suitable ones. In particular, we consider ranking- and separation-based measures, which emphasize the relative ordering of outputs and the degree of separation between correct and incorrect candidates. This aligns naturally with the design of Vatex-Eval, where the key objective is to reproduce the preference structure encoded in the averaged ratings rather than to match individual scores exactly.

\paragraph{LongVideoBench~\citep{wu2024longvideobenchbenchmarklongcontextinterleaved}}
To assess generalization to long-form videos (up to three minutes) and multiple-choice style evaluation, we repurpose the LongVideoBench dataset. We remove instructions requiring transcripts or involving ambiguous subtitle queries, and decompose each video–question pair into multiple instances, where the question and one candidate response are given as input. Models are prompted to rate each input, and performance is measured with two metrics. The first is the rating gap (\emph{Delta}) between correct and incorrect options, indicating whether correct answers receive consistently higher scores. The second is \emph{pairwise superiority}, the fraction of comparisons where the correct option is rated above distractors (ties counted half), averaged across questions. Together, these metrics capture both absolute preference for correct options and relative discrimination ability in the multiple-choice setting.

% Commenting it for now
% Most LLM-as-Judge evaluations are based on free-form generation. As a result, the models with poor instruction following get penalized. We follow the same and report instruction following accuracy along with other dataset-specific metrics. Instruction following accuracy is based on whether the generated response has a valid rating or not. For fair evaluation, we search exhaustively to extract the rating from the model response, irrespective of the format. As a result, we do not penalize models that do not follow a particular output format that we describe in the prompt. 

\subsubsection{Pairwise Evaluation}  
In pairwise evaluation, models are presented with two candidate responses for the same video--instruction and prompted to identify which response is better. This preference-style judgment allows us to measure accuracy against human or rating-based ground truth. By focusing on relative quality rather than absolute scores, pairwise evaluation provides a complementary perspective to pointwise evaluation.

\paragraph{VideoAutoArena~\citep{luo2025videoautoarenaautomatedarenaevaluating}}  
VideoAutoArena provides video-instruction pairs with two candidate responses, annotated with human preferences. We use human preference as ground truth and report accuracy.

\paragraph{VideoJudge-Pairwise}  
We derive pairwise evaluation data from our pointwise dataset by pairing responses with different ratings and designating the higher-rated response as the correct choice. Accuracy is reported with respect to this ground truth.  

\paragraph{VideoJudge-Pairwise-H}  
To assess performance on more challenging distinctions, we focus on pairs where responses are rated 2 vs.~3, a setting that is difficult even for humans due to subtle differences in specificity. From our pointwise data, we sample 250 such pairs and collect judgments from two human evaluators given the video, instruction, and responses. We retain only pairs with full agreement, yielding over 200 high-quality pairs with human preference as ground truth. Accuracy is reported as in other pairwise evaluations.
